# Supplementary material for: Self-Supervised Online Learning for Safety-Critical Control using Stereo Vision
Source: arXiv:2203.01404 source file (2022-03-02)
Supplement: Supplementary file 1 [file appendix.tex]

\appendix
\begin{theorem} \label{thm:robust_pixel_mrcbf}
% For $p \in N $ where $N$ is a finite subset of $\mathbb{N}$, let  $h_p: \R^n \to \R $ be a family of continuously differetiable functions with $0$ a regular value. Additionally, let $h_\textrm{ns} = \min_{p \in N} h_p(\mb{x}) $. 
% If $\mb{k}^*: \R^n \to \R^m$ is a locally-Lipschitz controller that satisfies \eqref{eq:safety_uncertain} for measurement $\widehat{\rho}_p \in \mathcal{E}(\rho_p)$, then the closed loop dynamics \eqref{eq:cl} are safe with respect to the set $\mathcal{C}_K$.
For $p \in K $ where $K$ is a finite subset of $\mathbb{N}^2$, let $h : \R^n \times \R^3 \to \R$ be a Lipschitz function with 0 a regular value. Define $h_\textrm{ns}(\mb{x}) \triangleq \min_{p \in K} h(\mb{x}, \rho_p) $. 
If $\mb{k}: \R^n \to \R^m$ is a locally-Lipschitz controller that satisfies \eqref{eq:safety_uncertain} with $\sigma =1$ for all measurements $\widehat{\rho}_p \in \mathcal{E}(\widehat{d}_p)$ and for all $\widehat{d}_p \in \mathtt{D}$, then the closed loop dynamics \eqref{eq:cl} are safe with respect to the set $\mathcal{C}_K$.
\end{theorem}

\begin{proof}
 First, we let $\widehat{h}_\textrm{ns}(\mb{x}) = \min_{p \in K} h(\mb{x}, \widehat \rho_p) $. We can then follow the main result of \cite{dean_guaranteeing_2020} and lower bound the left hand side of this inequality as follows: 
\begin{align}
        \min_{p \in \widehat\Lambda}& \; 
        % \frac{d}{dt}
        % \dot{h}_i (\mb{x}, \rho_i, u)
         \dot h (\mb{x}, \rho_p, \mb{k}(\mb{x}))
        + \gamma (h_\mathrm{ns}(\mb{x}))  \\
        & =  \min_{p \in \widehat \Lambda} \dot{h}(\mb{x}, \widehat{\rho}_p, \mb{k}(\mb{x}))  + \widehat h_\textrm{ns}(\mb{x})  \nonumber\\
        & \quad  + 
        \left( \dot{h}(\mb{x}, \rho_p, \mb{k}(\mb{x})) - \dot{h}(\mb{x}, \widehat{\rho}_p, \mb{k}(\mb{x}))\right) \nonumber\\
        & \quad + \left( h_\textrm{ns}(\mb{x}) - \widehat h_\textrm{ns}(\mb{x}) \right) \label{pf:add_zero}\\
        & \geq  \min_{p \in \widehat \Lambda} \dot{h}(\mb{x}, \widehat{\rho}_p, \mb{k}(\mb{x}))  + \widehat h_\textrm{ns}(\mb{x})  \nonumber \\
        & \quad -  \left( \mathfrak{L}_{L_fh} + \mathfrak{L}_{\gamma \circ h_\mathrm{ns}} + \mathfrak{L}_{L_gh} \Vert \mb{u } \Vert_2 \right) \epsilon_p \label{pf:Lipshitz}\\
        & \geq 0 \label{pf:controller_assp}.
\end{align}

In equation \eqref{pf:add_zero} we introduce $\widehat \rho_p $ by adding 0. Then we expand using the Lipschitz constants of each Lie derivative as well as the bound on error bound $\epsilon_p$. Also, minimizing a finite set of Lipschitz functions retains the Lipchitz property so $h_\textrm{ns}$ is Lipschitz. Since $\sigma = 1$ this bound holds with probability 1. Finally, the last inequality is due to the assumption that the controller $k$ satisfies \eqref{eq:safety_uncertain}. 

Next, we note that $\widehat \Lambda \supseteq \Lambda$ so 
\begin{align}
        \min_{p \in \widehat\Lambda} 
        % \frac{d}{dt}
        % \dot{h}_i (\mb{x}, \rho_i, u)
        \dot h (\mb{x}, \rho_p, \mb{k}(\mb{x}))  
        + \gamma (h_\mathrm{ns}(\mb{x})) \geq 0 
\end{align}
implies that \eqref{eq:safety_nonsmooth} must also be true. It follows immediately from Theorem \ref{thm:nonsmooth} that the closed loop system \eqref{eq:cl} is safe with respect to $\mathcal{C}_K$.

\end{proof}

% \begin{align*}
%     -v & \geq  \frac{\gamma (\min_{p \in K} h(\mb{x}, \rho_p^*))}{\lmat 1 & 0 & 0 \rmat^\intercal r(p,d_p^*) },  \forall p \in \widehat{ \Lambda} \\
%     & \implies  -v \geq  \frac{h_\textrm{ns}(\mb{x})}{\lmat 1 & 0 & 0 \rmat^\intercal r(p,d_p) },  \quad \forall p \in \widehat{ \Lambda}\\
%     & \implies  -v \geq  \frac{h_\textrm{ns}(\mb{x})}{\lmat 1 & 0 & 0 \rmat^\intercal r(p,d_p) },  \quad \forall p \in \Lambda\\
%     & \iff \dot{h} = -\lmat 1 & 0 & 0 \rmat^\intercal r(p,d_p)v \geq - \gamma(h(\mb{x})), \forall p \in \Lambda 
% \end{align*}
% since 

\newpage

% \section{New Barrier Function }
% \begin{equation}
%     h(\mb{x}_{rel}) = \frac{1}{2} \left( \Vert \mb{x}_{rel} \Vert^2  - \textrm{atan } \left(\frac{y_{rel}}{x_{rel}} \right)^2 - C^2 \right) 
% \end{equation}
